# Supplementary material for: Implicit Feature Decoupling with Depthwise Quantization
Source: arXiv:2203.08080 source file (2022-03-29)
Supplement: Supplementary file 2 [file rebuttal.tex]

\documentclass[10pt,twocolumn,letterpaper]{article}
\usepackage[rebuttal]{cvpr}

% Include other packages here, before hyperref.
\usepackage{graphicx}
\usepackage{amsmath}
\usepackage{amssymb}
\usepackage{booktabs}


% If you comment hyperref and then uncomment it, you should delete
% egpaper.aux before re-running latex.  (Or just hit 'q' on the first latex
% run, let it finish, and you should be clear).
\usepackage[pagebackref,breaklinks,colorlinks,bookmarks=false]{hyperref}

% Support for easy cross-referencing
\usepackage[capitalize]{cleveref}
\crefname{section}{Sec.}{Secs.}
\Crefname{section}{Section}{Sections}
\Crefname{table}{Table}{Tables}
\crefname{table}{Tab.}{Tabs.}

% If you wish to avoid re-using figure, table, and equation numbers from
% the main paper, please uncomment the following and change the numbers
% appropriately.
%\setcounter{figure}{2}
%\setcounter{table}{1}
%\setcounter{equation}{2}

% If you wish to avoid re-using reference numbers from the main paper,
% please uncomment the following and change the counter for `enumiv' to
% the number of references you have in the main paper (here, 6).
%\let\oldthebibliography=\thebibliography
%\let\oldendthebibliography=\endthebibliography
%\renewenvironment{thebibliography}[1]{%
%     \oldthebibliography{#1}%
%     \setcounter{enumiv}{6}%
%}{\oldendthebibliography}


%%%%%%%%% PAPER ID  - PLEASE UPDATE
\def\cvprPaperID{9244} % *** Enter the CVPR Paper ID here
\def\confName{CVPR}
\def\confYear{2022}

\begin{document}

%%%%%%%%% TITLE - PLEASE UPDATE
\title{Implicit Feature Decoupling with Depthwise Quantization}

\maketitle
\thispagestyle{empty}
\appendix
We would like to thank the reviewers for their valuable feedback. We are glad to see that our work was found to be well organized with sufficient experimental results that verify the usefulness of our method.

\textbf{Response to Reviewer 1}
\textit{The authors \dots representation.}

The reviewer has correctly pointed out that we limit the qualitative evaluation on the disentangled representations and only show the codebook utilization for different hierarchies such as in Fig. 4 of the main text. To evaluate the disentangled representations in a similar context as a $\beta$-VAE would require interpolating along the discretized latent space and does not lead 
to meaningful reconstructions. 
Interpolating requires sampling using an auxiliary model trained on the quantization codes. There are additional challenges in designing an auxiliary model for interpolating in the quantized latent space that is specific to our method and consider it a good future work. We plan to revise our paper to add details of this remark in the Discussion section for a camera-ready version. 

%Quantitatively, we verify our claim on disentangled representations using Entropy and Mutual Information between codes. Finally, we do agree that Fig 4. can be improved and will address it in a camera-ready version. 

\textit{The authors state $\dots$ the optimiser play?} The reviewer has correctly pointed out that the relationship between our method, VAE, and EMA is not clear solely from the work done by Kaiser \etal[19]. We plan to supplement our analysis in a camera-ready version. 

There is no \textit{exact} relationship between $\beta$ parameter and the EMA parameters or the weight decay of the optimizer. DQ is an approximation to the Varitional Information Bottleneck (VIB) \cite{roy2018towards} when trained with soft Expectation-Maximization (EM) which is a consequence of using EMA \cite{on_line_em,chen2018stochastic}. 
Additional detailed analysis can be found in the work by Wu \etal\cite{wu2018variational}.
%In contrast to hard EM where quantization is deterministic \cite{roy2018theory}. 

\textit{I couldn’t find an $\dots$ illustrated in figure 5.} We agree with the reviewer that the connection between Table 2 and Figure 5 of the main text is confusing. We will provide an improved explanation of the difference between the two experiments for a camera-ready version. The loss reported in Table 2 is calculated using $L_{DQ}$ from Eq. 4 in the main text and is calculated on a \textit{static prior}. Contrary to Fig. 5 where  we report the reconstruction loss $L_\text{DNN}$ from Eq. 5 on a \textit{learned prior}. 

\textit{The authors describe the use of EMA \dots} We use Eq. 9 in the work by Kaiser \etal[19] and in our code corresponds to line 47 of the file dq.py. % in the \textit{\_update\_embed} function.

\textit{An alternative means \dots} Lastly, we would like to thank the reviewer for referencing MINE %\cite{belghazi2018mine} 
which is useful for estimating the mutual information between high-dimensional continuous variables, in contrast to our method which is used for quantized representations. We plan to supplement with a comparison in the Related Works section for a camera-ready version.


\textbf{Response to Reviewer 2} \textit{1. In line 477 $\dots$ provided.} This was not explained clearly enough and we will emphasize it on the camera-ready version. We compare DQ to a $\beta$-VAE and provide a theoretical justification on the advantage of DQ in Sec. 4.1.  In Sec. 4.2 we draw a parallel with the feature decomposition approaches (DSC  [7,39]) and (BSConv [14]) that are applied on the axis of weak statistical dependence. We experimentally verify our claim in Sec. 5.2 \textit{Implicit Decoupling}

\textit{2. In the experiment, the authors do not mention \dots} The reviewer has correctly pointed out that we do not have details on the random seed methodology and we will address it for a camera-ready version. We did not set the random seed to a fixed value but instead, we used a random seed at every trial. %such that the parameter initialization is truly random. 

\textit{3. The evaluation results of DQ on other ...}The reviewer has correctly pointed out that we only evaluate our method on CIFAR-10 and 2 resolutions of ImageNet. We choose CIFAR10 that is complex to show significant differences and small in size which make it feasible to perform the ablation study experiments. ImageNet is reported by all our baselines. %\cite{child2019generating, parmar2018image,vdvae} 
%and is standardized large size dataset. 
We perform additional experiments on MNIST %\cite{lecun-mnisthandwrittendigit-2010} 
where DQ (``Our'') out-performed VQ with 1.92e-04 in $l_2$ reconstruction loss as compared to 3.41e-04 and similarly for CelebA %\cite{liu2015faceattributes} 
with 9.57e-03 compared to 3.70e-02. For reasons of brevity in our response, we will supplement the camera-ready version with additional results on Tab. 2 in the Appendix and with qualitative results similar to Fig. 4 for the datasets mentioned.

\textit{4. In contrast to the $\dots$.}
The reviewer has correctly pointed out that the explanation on the poor assumption of quantization methods with a uniform prior can be improved and we will address it for a camera-ready version. A prior that is not uniform can be quantitatively observed with \textit{codebook collapse}. In our method, we resolve \textit{codebook collapse} with the use of EMA and random re-initialization of codes [19]. We address the issue in better detail in Sec 4.2 \textit{Uniform Prior} and our second response to Reviewer 1. 


%%%%%%%%% REFERENCES
{\small
\bibliographystyle{ieee_fullname}
\bibliography{bib_main}
}

\end{document}
